# Supplementary material for: Controlling Face's Frame generation in StyleGAN's latent space operations: Modifying faces to deceive our memory
Source: arXiv:2407.00803 source file (2024-06-30)
Supplement: Supplementary file 1 [file Appendix.tex]

\documentclass[../00_Main.tex]{subfiles}
\begin{document}

TODO: No entiendo que iría acá

\biblio % Needed for referencing to working when compiling individual subfiles - Do not remove
\end{document}
